# Supplementary material for: MILR: Mathematically Induced Layer Recovery for Plaintext Space Error Correction of CNNs
Source: arXiv:2010.14687 source file (2020-10-28)
Supplement: Supplementary file 1 [file appendix.tex]

\section{Appendix A: Handling of Other Layers}

Dense and convolutional layers are discussed in the main paper. This appendix discusses the handling of other layers.  

\

\section{Appendix B: CRC Evaluation}
