# Supplementary material for: MILR: Mathematically Induced Layer Recovery for Plaintext Space Error Correction of CNNs
Source: arXiv:2010.14687 source file (2020-10-28)
Supplement: Supplementary file 2 [file appendixC.tex]

% Moved into Paper

\section{Appendix C: MILR Evaluation}
\input{tables/network}

Our testing was done on two networks (MNIST~\cite{LeCun2005TheMD} and CIFAR-10~\cite{Krizhevsky2009LearningML}), with details shown in Table~\ref{tab:MNIST} and~\ref{tab:cifar}. We perform three types of experiments: (1) inject bit errors a probability of \(p\) (i.e. Raw Bit Error Rates (RBER)), (2) inject whole-weight errors with a probability of \(q\), and (3) corrupt entire layers. For experiments (2) and (3), ECC is unable to recover from errors, while MILR can in many cases. For the MNIST network experiment (1) was presented in the main paper and will be summarized here, and experiments (2) and (3) will be fully presented. For the CIFAR network experiments (1),(2), and (3) will be presented as a only a summary was given in the main paper. 

\subsection{MNIST Network}
The MNIST handwritten numbers database \cite{LeCun2005TheMD} is a commonly used database in machine learning, with 60,000 28 x 28 black and white training images and 10,000 images for testing; which are classified into 10 categories. The network was built according to table \ref{tab:MNIST}, with valid padding convolution layers, and a bias and ReLu activation layer after each dense and convolution layer. The network was trained for 5 epochs with a batch size of 128, to an accuracy of \(99.2\%\).

Figure~\ref{fig:MNIST-ACC} shows box plots of 40 runs with varying RBER with normalized average accuracy (i.e. 100\% means the same accuracy as the error-free version). Figure~\ref{fig:MNIST_error} shows the raw un-recovered effect of the RBER, with figures \ref{fig:MNSIT_ecc}, and \ref{fig:MNIST_recov}, and \ref{fig:mnist_eccMilr} showing the accuracy after error is detected and recovered using ECC and MILR, and a combination of ECC and MILR (ECC+MILR). Each plot is centered on the median values, with the box covering the \(25^{th}\) and \(75^{th}\) percentile (i.e. {\em interquartile} range). The whiskers extended \(1.5\times\) the interquartile range from the top and bottom of the box, up to the max/min value. Outliers are marked by dots on the graph. The mean value is summarized for each graph in Table~\ref{tab:MNIST_acc}.

\begin{scriptsize}
    \begin{table*}[htbp]
        \centering
        \caption{MNIST network RBER accuracy }
        \label{tab:MNIST_acc}
        \begin{tabular}{|l|l|l|l|l|l|l|l|l|l|}
            \hline
            \textbf{Recovery} & \textbf{1E-07} & \textbf{5E-07} & \textbf{1E-06} & \textbf{5E-06} & \textbf{1E-05} & \textbf{5E-05} & \textbf{1E-04} & \textbf{5E-04} & \textbf{1E-03}\\
            \hline
            \hline
            None & 99.1\% &	94.3\% &	85.6\% &	58.9\% &	37.8\% &	12.9\% &	12.9\% &	10.0\% &	10.1\%\\
            \hline
            ECC &   100.0\% &	100.0\% &	100.0\% &	100.0\% &	100.0\% &	99.5\% &	97.0\% &	43.5\% &	14.8\%\\
            \hline
            MILR &  100.0\% &	100.0\% &	100.0\% &	100.0\% &	98.7\% &	100.0\% &	99.0\% &	89.3\% &	73.2\%\\
            \hline
            ECC + MILR & 100.0\% &	100.0\% &	100.0\% &	100.0\% &	100.0\% &	100.0\% &	100.0\% &	100.0\% &	98.4\%\\
            \hline
        \end{tabular}
    \end{table*}
\end{scriptsize}
\input{diagrams/MNIST_graphs}

The MINST network does have some intrinsic robustness achieving \(99.2\%\) of  accuracy with an error rate of \(1E-07\), when injected with bit errors. ECC maintains \(100.0\%\) of accuracy to  \(1E-05\) as it corrects all single bit errors. MILR was able to achieve \(100.0\%\) accuracy through \(5E-05\), which beat out ECC. This performance is due to the ability to address multi-bit errors that start appearing after \(5E-06\). ECC + MILR was able to achieve \(100.0\%\) accuracy throughout the test range, this is due to ECC addressing all of the single bit errors then only leaving the less common multi-bit errors to MILR. This reduction of errors when it reaches MILR reduces the chances of multiple erroneous layers between checkpoint pairs. 

\begin{scriptsize}
    \begin{table*}[htbp]
        \centering
        \caption{MNIST network whole-weight errors accuracy  }
        \label{tab:MNIST_acc_wholeWord}
        \begin{tabular}{|l|l|l|l|l|l|l|l|l|l|l|}
            \hline
            \textbf{Recovery} & \textbf{1E-07} & \textbf{5E-07} & \textbf{1E-06} & \textbf{5E-06} & \textbf{1E-05} & \textbf{5E-05} & \textbf{1E-04} & \textbf{5E-04} & \textbf{1E-03} & \textbf{5E-03}\\
            \hline
            \hline
            None & 100.0\% &	97.3\% &	96.6\% &	85.1\% &	68.0\% &	26.4\% &	13.1\% &	10.7\% &	10.0\% &	10.0\% \\
            \hline
            MILR  & 100.0\% &	100.0\% &	100.0\% &	100.0\% &	100.0\% &	100.0\% &	100.0\% &	99.9\% &	94.6\% &	55.9\% \\
            \hline
        \end{tabular}
    \end{table*}
\end{scriptsize}
\input{diagrams/MNIST_WHOLE}
The MNIST network was also tested with whole-weight errors with a probability of \(q\), where every bit in a word was flipped. ECC and ECC + MILR were not tested with this scheme as ECC can only correct 1 bit errors and all errors injected would be 32 bit errors. The network still had some intrinsic robustness with having at least \(99\%\) of accuracy through an error rate of \(5E-07\). When MILR is applied it is able to recover the network to \(100.0\%\) accuracy through \(1e-05\). After this point, multiple erroneous layers between checkpoint  pairs start to appear, starting to affect the recovery accuracy.

To test a scenario when a whole layer is erroneous each layer individually has all of its parameters replaced by a random values, where none of the values were the same as the original value. Then MILR attempted to solve the layers back to it's original state. For the convolution layers using the two dimensional CRC for partial recoverability, they by design could not recovery the full layer. In those scenarios, they followed their standard recovery process but when they attempt to solve their system of equation they have more variables than equations. To address this they attempt to find a least-square solution. This provides a solution to the linear equation as close as possible to the actual solution. The less under-defined the problem the close the solution should be, however the precision will vary. If the system of equation is to underdefined the system is not solvable even by finding the least-square solution. In these cases no recovery is possible, however the probability of these cases is slim.  Also in this test, the bias of a layer is considered as separate layer and is treated as such. 
\input{tables/MNIST_WholeLayer}

Whole layer errors showed that each layer is important to the network serving a purpose. The main function of the layer is of key performance, with the bias layer serving less but still playing a significant role. The bias layers of the dense layers had the least affect on the network compared to other layers. For recovery MILR was able to recovery all layers to a usable state beside one of the convolution layers. This layer used two dimensional CRC for partial recoverability, making it hard to be fully recovered.

\subsection{CIFAR-10 Network}
The Cifar-10 database \cite{Krizhevsky2009LearningML} is a color image database with 60,000 \(32\times 32\)  images, that can be categorized into 10 categories with 6,000 examples of each in the database. The database is partitioned into 50,000 images for training and 10,000 for testing. The network was built according to table \ref{tab:cifar} with same padding convolution layers, and a bias and ReLu activation layer after each dense and convolution layer. The architecture of the network was inspired by the VGG network \cite{Simonyan2015VeryDC}, but minus the last few layers as we not using the Imagenet database \cite{ILSVRC15}. The CIFAR-10 network was trained to \(71.3\%\) accuracy, over 75 epochs with a batch size of 32.
\begin{scriptsize}
    \begin{table*}[htbp]
        \centering
        \caption{CIFAR-10 small network RBER accuracy }
        \label{tab:CIFAR_acc}
        \begin{tabular}{|l|l|l|l|l|l|l|l|l|}
            \hline
            \textbf{Recovery}  & \textbf{ 1E-07}  & \textbf{5E-07}  & \textbf{1E-06}  & \textbf{5E-06}  & \textbf{1E-05}  & \textbf{5E-05}  & \textbf{1E-04}& \textbf{5E-04}\\
            \hline
            \hline
            None &  99.1\% &	81.5\% &	70.5\% &	24.2\% &	13.6\% &	12.0\% &	11.8\% &	11.7\%\\
            \hline
            ECC &   100.0\% &	100.0\% &	100.0\% &	100.0\% &	100.0\% &	97.8\% &	82.4\% &	16.9\%\\
            \hline
            MILR &  100.0\% &	100.0\% &	100.0\% &	100.0\% &	100.0\% &	98.8\% &	95.4\% &	80.2\%\\
            \hline
            ECC + MILR &   100.0\% &	100.0\% &	100.0\% &	100.0\% &	100.0\% &	100.0\% &	100.0\% &	100.0\% \\
           \hline
        \end{tabular}
    \end{table*}
\end{scriptsize}

\input{diagrams/CIFAR_graph}

The CIFAR-10 network  without any recovery has less robustness compared to the MNIST network only achieving \(91.1\%\) of accuracy at \(1E-07\), when injected with bit flips with the same probability. This shows that the network has a higher sensitivity to bit flips. ECC is able to maintain \(100.0\%\) of performance up to \(1E-05\), matching the same performance as the MNIST network. This is due to the probability of multi-bit errors staying the same regardless of the network structure.

MILR was able to achieve a \(100.0\) of accuracy up to \(1E-06\). However, it did drop below this point at lower error rate of \(5E-07\). This is due to the increase in layer size of the network. With larger layer sizes, each layer is more susceptible to errors. Increasing the probability of multiple erroneous layer between a pair of checkpoints. Also with larger layer sizes the limitation of the 32-bit float appear more. As most parameters are \([1,-1]\) the precision of the representation can and rounding error in solve systems of equations can lead to less precise recoveries. 
\input{tables/CIFAR_64_acc}
\input{diagrams/CIFAR-Graph-64}

Testing the same network with 64-bit parameter representation the MILR performance stayed approximately the same achieving \(99.9\%\) of accuracy to \(1E-06\). But the drop off of MILR performance is decreased as rounding precision errors due to the floating point representation can be reduced. MILR still runs into the issue of multiple erroneous layer between checkpoints, but the performance in those situations still is increased.

For the CIFAR-10 network MILR detected all erroneous layers in \(76.5\%\) of the test at our above the \(R(.999)\) error rate of \(1E-06\), with injected bit errors. In the test in which not all erroneous layers were detected \(97.9\%\) of the test had their accuracy restored to \(99.9\%\) of the non-erroneous accuracy.  
\begin{scriptsize}
    \begin{table*}[htbp]
        \centering
        \caption{CIFAR-10 small network whole-weight errors accuracy }
        \label{tab:CIFAR_acc_wholeword}
        \begin{tabular}{|l|l|l|l|l|l|l|l|l|l|}
            \hline
            \textbf{Recovery} & \textbf{1E-07} & \textbf{5E-07} & \textbf{1E-06} & \textbf{5E-06} & \textbf{1E-05} & \textbf{5E-05} & \textbf{1E-04}& \textbf{5E-04}& \textbf{1E-03}\\
            \hline
            \hline
            None &  97.5\% &	87.8\% &	83.6\% &	49.5\% &	25.4\% &	11.8\% &	11.4\% &	11.8\% &	11.7\% \\
            \hline
            MILR &  100.0\% &	100.0\% &	100.0\% &	100.0\% &	100.0\% &	100.0\% &	100.0\% &	97.7\% &	92.0\% \\
            \hline
        \end{tabular}
    \end{table*}
\end{scriptsize} 

When tested with whole-weight errors the network still had some intirsic robustness, achieving \(99.2\%\) of accuracy at an error rate of \(1E-07\). ECC was not tested as ECC's performance would match the no recovery performance, as all errors were 32 bits. MILR was able to keep \(100.0\%\) of accuracy to \(1E-05\) as after this point multiple erronous layers between checkpoints stated to appear. This performance shows were MILR is most capable large errors densely arranged, and where it beats out ECC's correcting ability. 
\input{tables/CIFAR_WholeLayer}

The CIFAR-10 network with full layer errors had similar results to the MNIST network. It did have more partial recoverable layers, however due to the degree in which they were under-defined they could not be solved, thus giving no recovery results. The dense bias layers also ran into issues on recovery. Due to the 32 bit representation the precision of the value was not maintained. Usually the bias \([-1,1]\), but due to the effect of the 32 bit representation the value recovered was significantly greater than \(1\). This is supported by how the effect of the bias with errors was minimal, as for the most part the effects of bias would be rounded out my the 32 bit representation. 

\input{tables/CIFAR_storage}

The CIFAR network's hyperparameters allowed for a lower storage overhead as it allowed for more data reuse. To store a second copy of the network it would cost 11.15 MB of storage. MILR only cost 8.66 MB of additional storage a \(22\%\) reduction in storage overhead. ECC is still cheaper only cost 2.42 MB, but still susceptible to multi-bit errors.  Combining ECC and MILR allows for all scenarios to be covered with single bit errors being handled by ECC and multi-bit errors being handled by MILR while costing less then storing a second copy of the network.
